# Supplementary material for: Differentially Private Synthetic Mixed-Type Data Generation For Unsupervised Learning
Source: arXiv:1912.03250 source file (2020-12-10)
Supplement: Supplementary file 1 [file appendix-NIST.tex]

\subsection{Additional Differentially Private Data Generation Algorithms}
In Section \ref{sec:related-work}, we discuss prior work on private synthetic data generation. In this section, we include other empirical work in this area.
\paragraph{NIST challenge on 1940 census data.} Five algorithms that generates synthetic data for the mixed-type 1940 census data are publicly available \cite{NIST2018Match3}. However, due to diverse approaches to preprocess the data and some steps in many of these algorithms tailored to this specific data and evaluation metrics used for the challenge, it is inappropriate, if not impossible, to use any of these algorithms as baseline applying to other datasets such as ones we use in this paper.
