# Supplementary material for: Differentially Private Synthetic Mixed-Type Data Generation For Unsupervised Learning
Source: arXiv:1912.03250 source file (2020-12-10)
Supplement: Supplementary file 2 [file appendix-metric.tex]

% \section{More Details on Metric}\label{app.metric}
% PCA algorithm metric
